# Supplementary material for: Neural Logic Reasoning
Source: arXiv:2008.09514 source file (2020-08-20)
Supplement: Supplementary file 1 [file appendix.tex]

\newpage
\onecolumn
\section*{APPENDIX}

To help understand the training process, we showing the changing curve of Traing/Validation/Testing RMSE during the training process on simulation data in Figure~\ref{fig:training_epoch_rmse}. 

\begin{figure}[htbp]
    \centering
    % \fbox{\rule[-.5cm]{0cm}{4cm} \rule[-.5cm]{4cm}{0cm}}
    \includegraphics[width=1.0\linewidth,trim={0 0mm 0 0mm},clip]{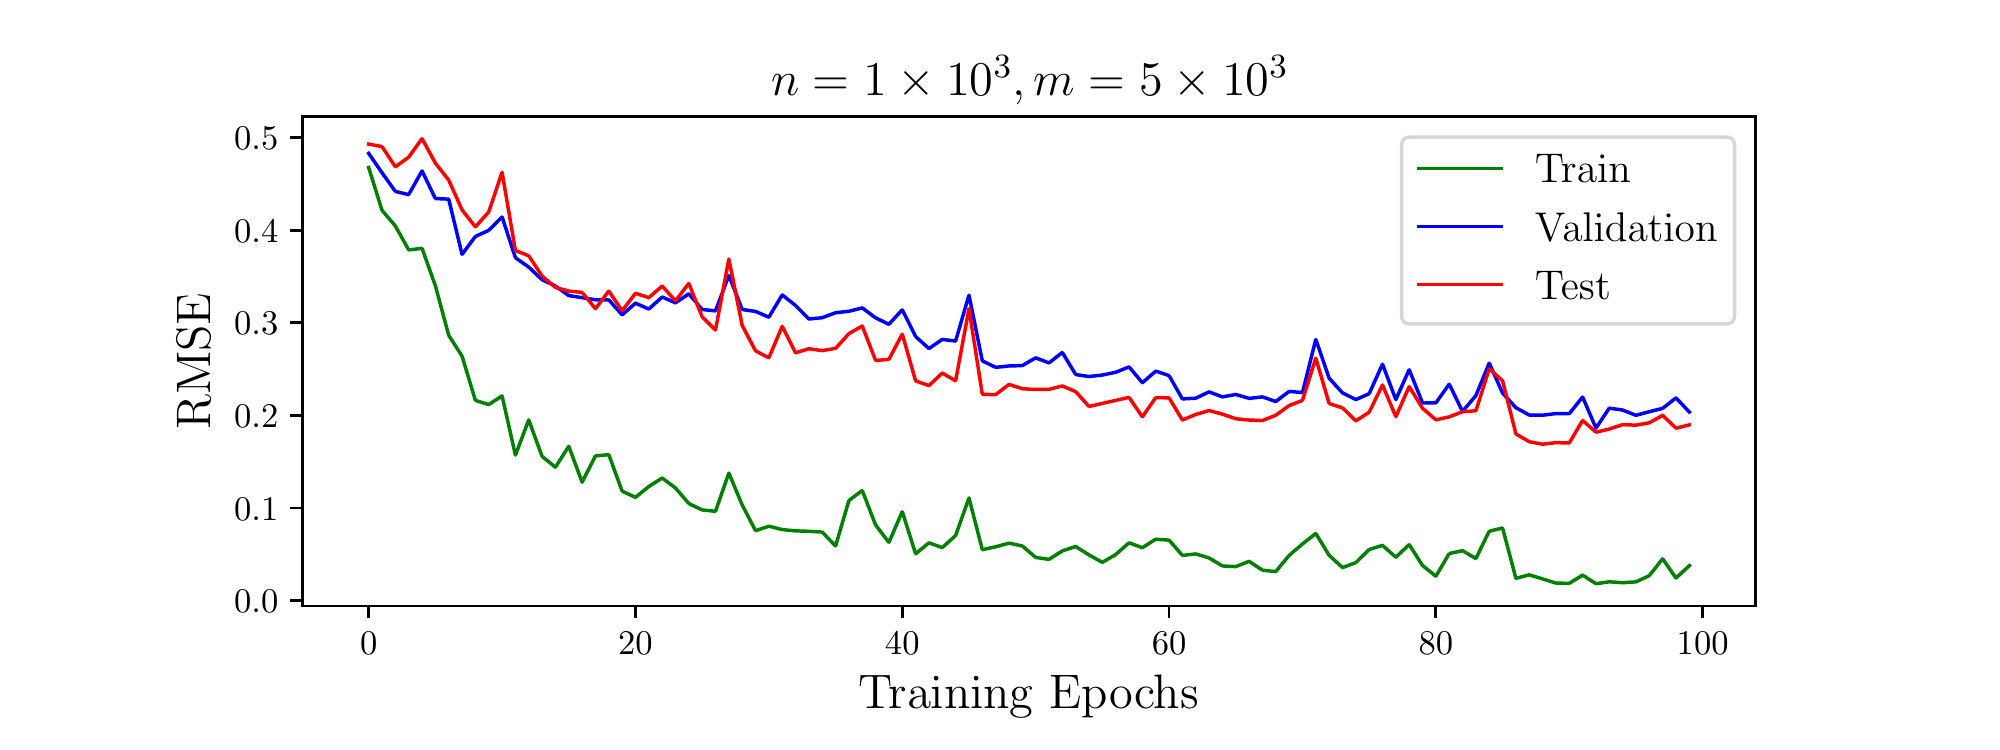}
    \vspace{-3mm}
    \caption{Changing curve of RMSE during the training process.}
    \label{fig:training_epoch_rmse}
\end{figure}

Furthermore, the visualization of variable embeddings in different epochs are shown in Figure~\ref{fig:training_epoch_variable_tsne}.

\begin{figure}[htbp]
    \centering
    % \fbox{\rule[-.5cm]{0cm}{4cm} \rule[-.5cm]{4cm}{0cm}}
    \includegraphics[width=0.5\linewidth,trim={0 0mm 0 0mm},clip]{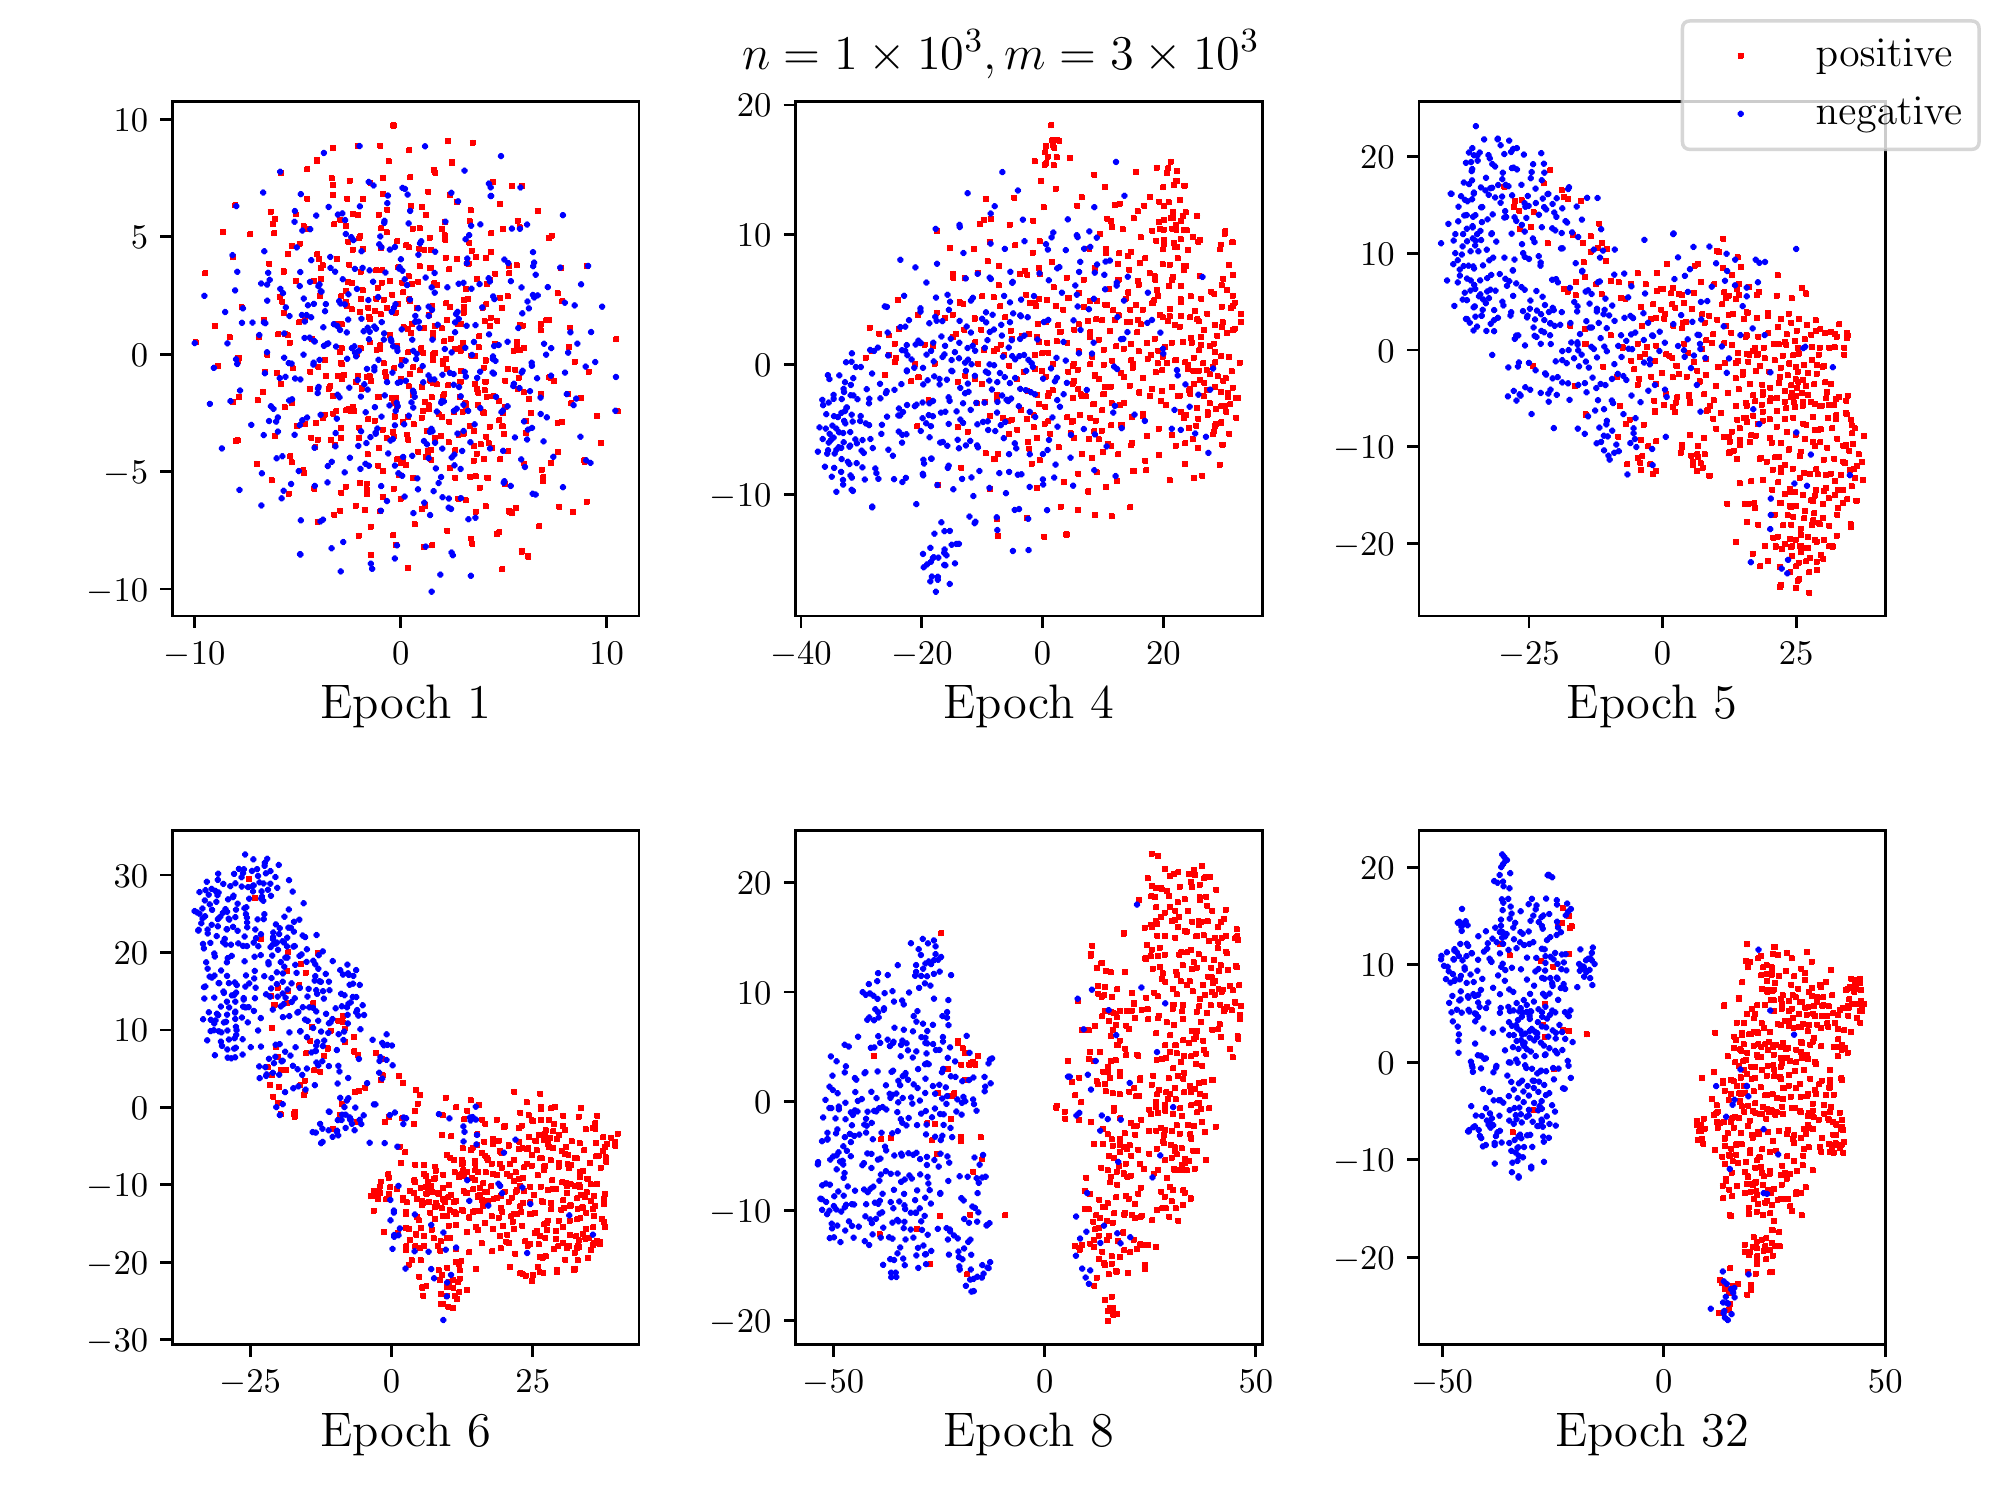}
    \vspace{-3mm}
    \caption{Visualization of variable embeddings in different epochs with t-SNE.}
    \label{fig:training_epoch_variable_tsne}
\end{figure}
